# Supplementary material for: Feedback RoI Features Improve Aerial Object Detection
Source: arXiv:2311.17129 source file (2023-11-28)
Supplement: Supplementary file 1 [file X_suppl.tex]

\clearpage
\setcounter{page}{1}
\maketitlesupplementary

% \section{Rationale}
% \label{sec:rationale}
% % 
% Having the supplementary compiled together with the main paper means that:
% % 
% \begin{itemize}
% \item The supplementary can back-reference sections of the main paper, for example, we can refer to \cref{sec:intro};
% \item The main paper can forward reference sub-sections within the supplementary explicitly (e.g. referring to a particular experiment); 
% \item When submitted to arXiv, the supplementary will already included at the end of the paper.
% \end{itemize}
% % 
% To split the supplementary pages from the main paper, you can use \href{https://support.apple.com/en-ca/guide/preview/prvw11793/mac#:~:text=Delete%20a%20page%20from%20a,or%20choose%20Edit%20%3E%20Delete).}{Preview (on macOS)}, \href{https://www.adobe.com/acrobat/how-to/delete-pages-from-pdf.html#:~:text=Choose%20%E2%80%9CTools%E2%80%9D%20%3E%20%E2%80%9COrganize,or%20pages%20from%20the%20file.}{Adobe Acrobat} (on all OSs), as well as \href{https://superuser.com/questions/517986/is-it-possible-to-delete-some-pages-of-a-pdf-document}{command line tools}.

\section{Implementation Details}
For all experiments, we follow the training protocols described in the original papers for each base model unless specified otherwise.

For ReDet\cite{han2021redet} and RoI Transformer\cite{ding2019learning}, in all datasets, we use a learning rate of 0.01, momentum of 0.9, and weight decay of 0.0001 when using SGD. For Rotated Faster R-CNN, in the DOTA-v1.0 dataset, we use a learning rate of 0.01, momentum of 0.9, and weight decay of 0.0001 when using SGD. For DOTA-v1.5 and HRSC2016, we use Adam with a learning rate of 0.0001 and a weight decay of 0.01. For Gliding Vertex \cite{xu2020gliding}, we use Adam with a learning rate of 0.0001 and a weight decay of 0.01. For DOTA-v1.0 and DOTA-v1.5, we train models with 12 epochs, reducing the learning rate 10-fold at epoch 8 and epoch 11, respectively. For HRSC2016, we train models with 36 epochs, reducing the learning rate 10-fold at epoch 24 and epoch 33, respectively. 

For Faster R-CNN and Mask R-CNN in our experiments on the MS COCO\cite{lin2014microsoft}, we employ an SGD optimizer with a learning rate of 0.02, momentum of 0.9, and weight decay of 0.0001.

\section{Additional Qualitative Results}

We include further visualizations of our method's detection results in \cref{fig:main2}. The first two rows show detection results from ReDet and ReDet + \model on clean images, and the last two rows show detection results from ReDet and ReDet + \model on blurred images.

We observe that the original ReDet tends to give false detections on blurred images, and incorporating \model improves these errors. For instance, in the second column of \cref{fig:sub1}, the airport terminal is misidentified as an airplane in the third row (ReDet on blurred image). ReDet+\model, on the other hand, does not make such a mistake on blurred images in the fourth row. In the third and fourth columns, we observe similar errors and improvements for the soccer ball fields (SBF). On the other hand, blurring may cause Redet to miss detections that were successful in the original images (first column, \cref{fig:sub3}) while adding \model helps to recover those detections.

\begin{figure*}[ht]
    \centering
    \begin{subfigure}{0.99\textwidth}
        \includegraphics[width=\textwidth]{figures/flex_vis11.png}
        \caption{}
        \vspace{0.43cm}
        \label{fig:sub1}
    \end{subfigure}
    \label{fig:main1}
\end{figure*}

\begin{figure*}[b]
    \ContinuedFloat
    \centering
    \begin{subfigure}{0.99\textwidth}
        \includegraphics[width=\textwidth]{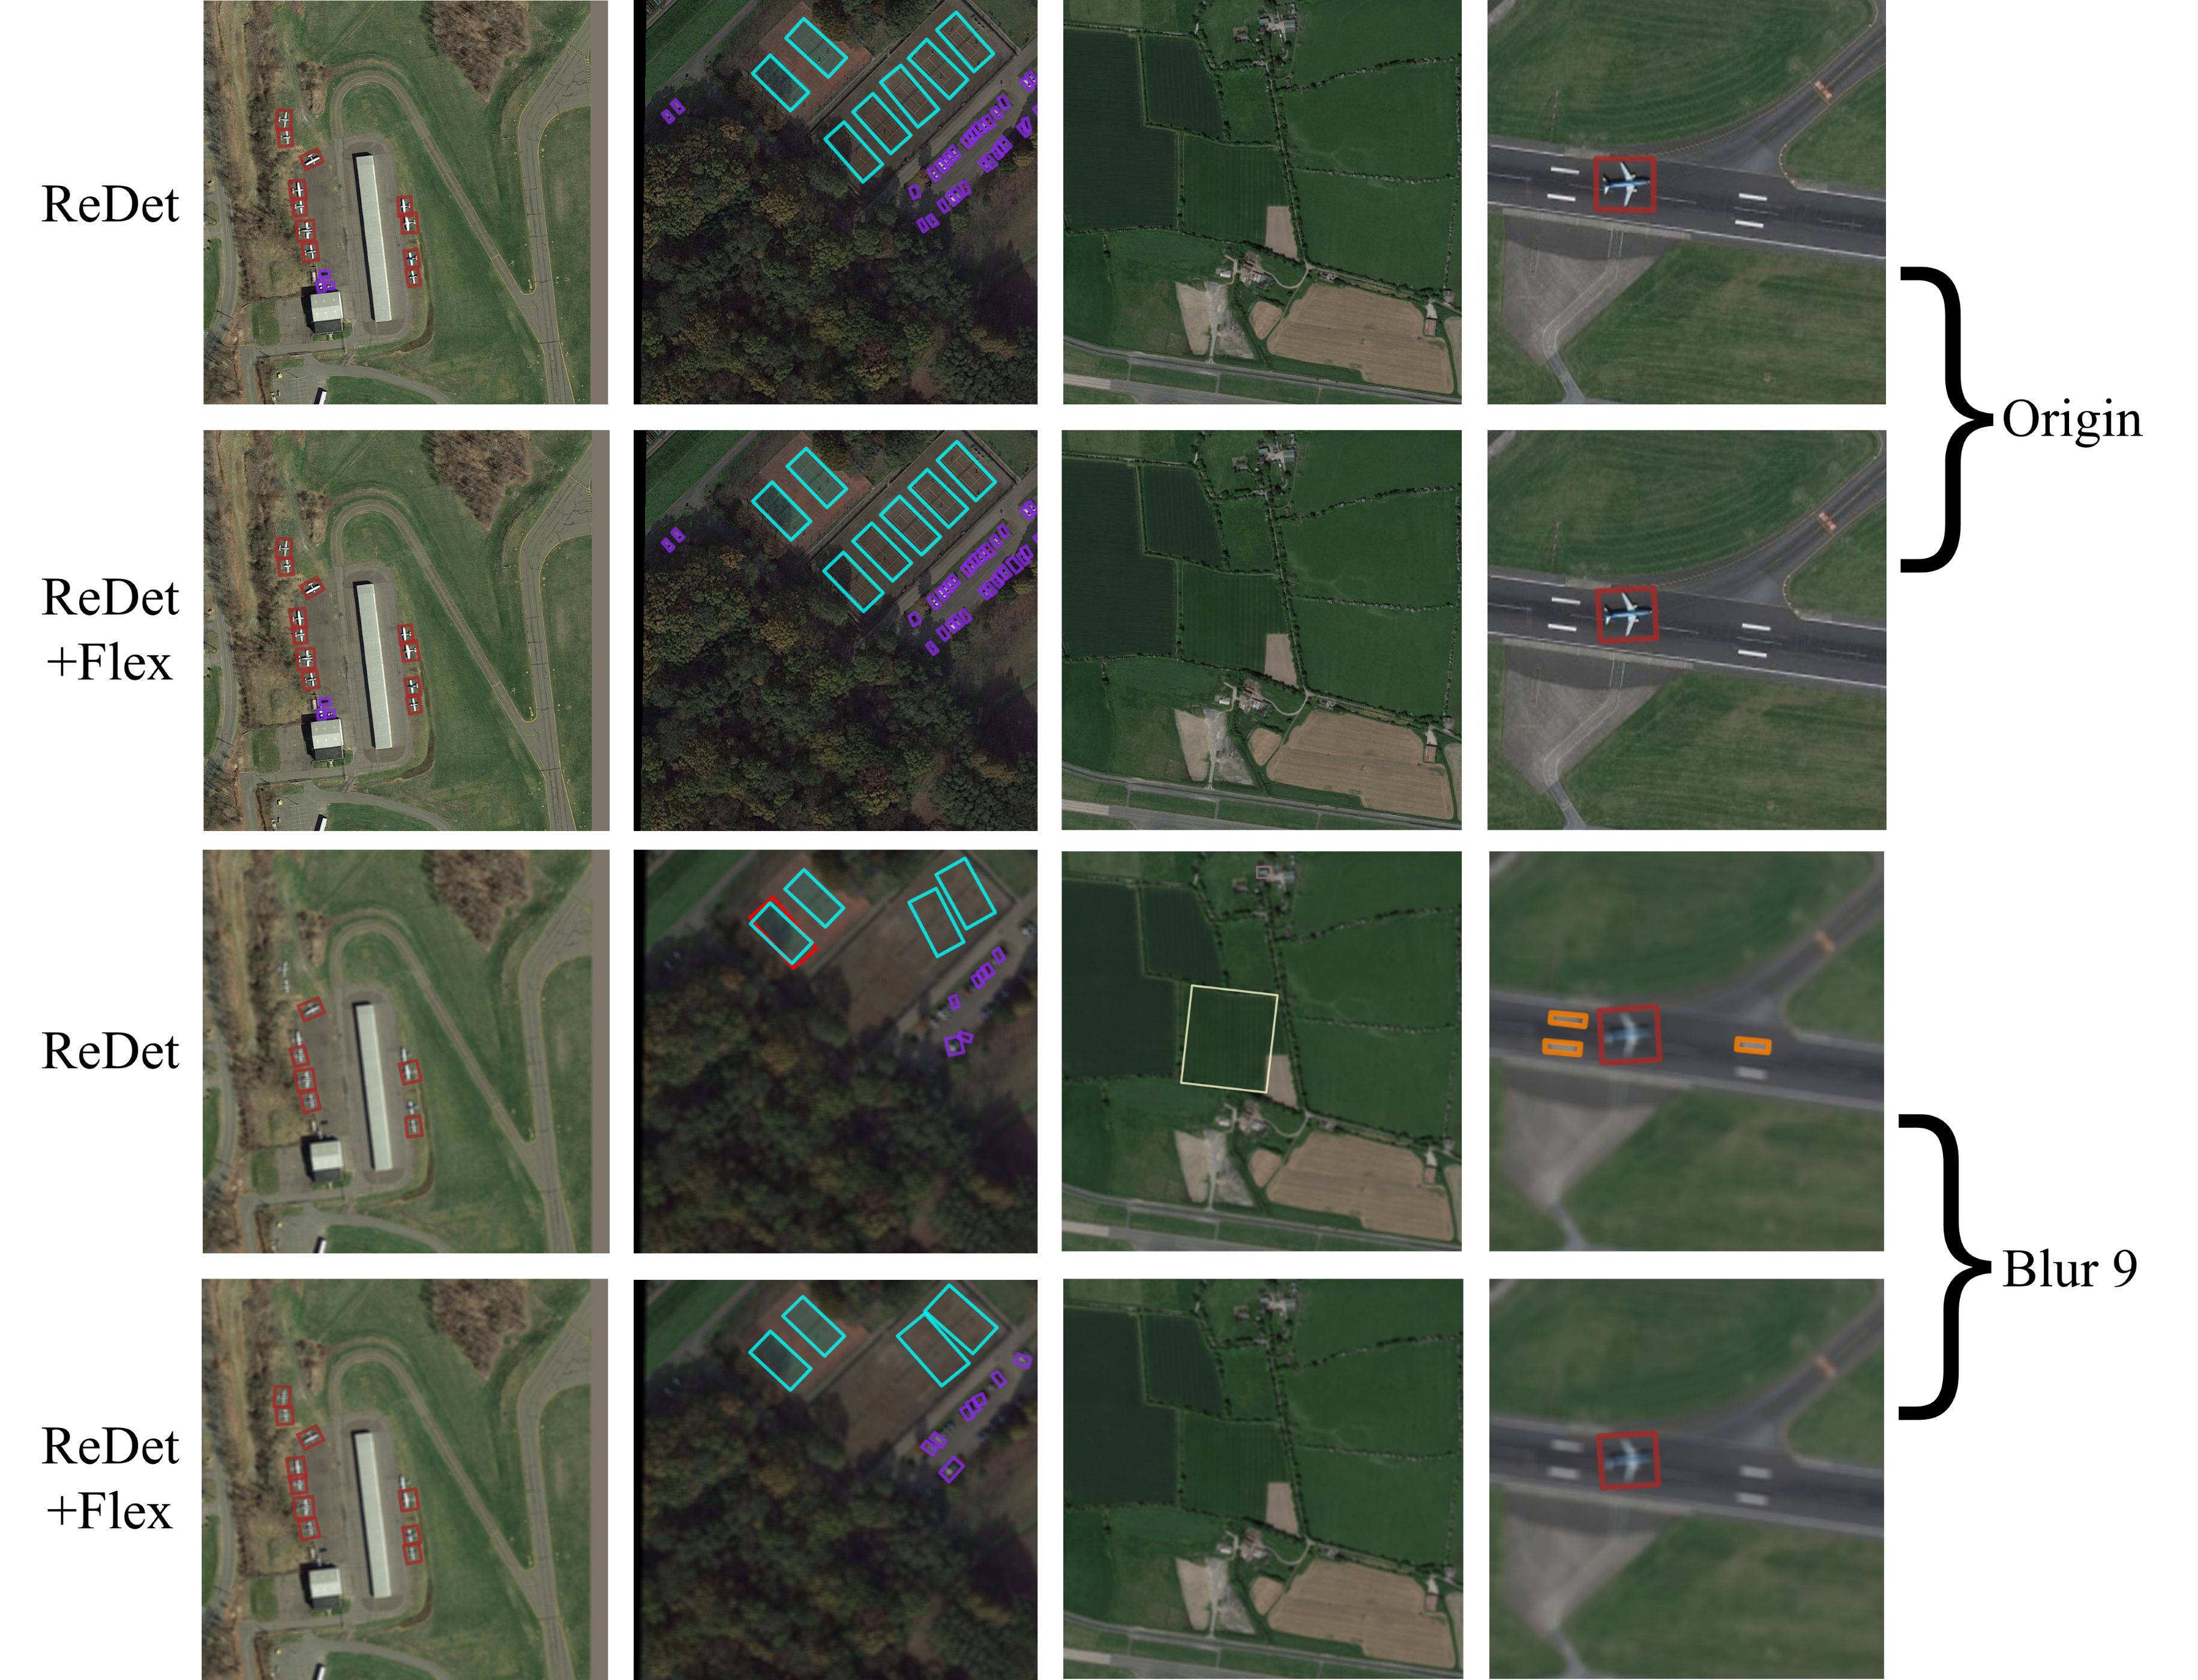}
        \caption{}
        \vspace{0.43cm}
        \label{fig:sub3}
    \end{subfigure}
    \begin{subfigure}{0.7\textwidth}
        \includegraphics[width=\textwidth]{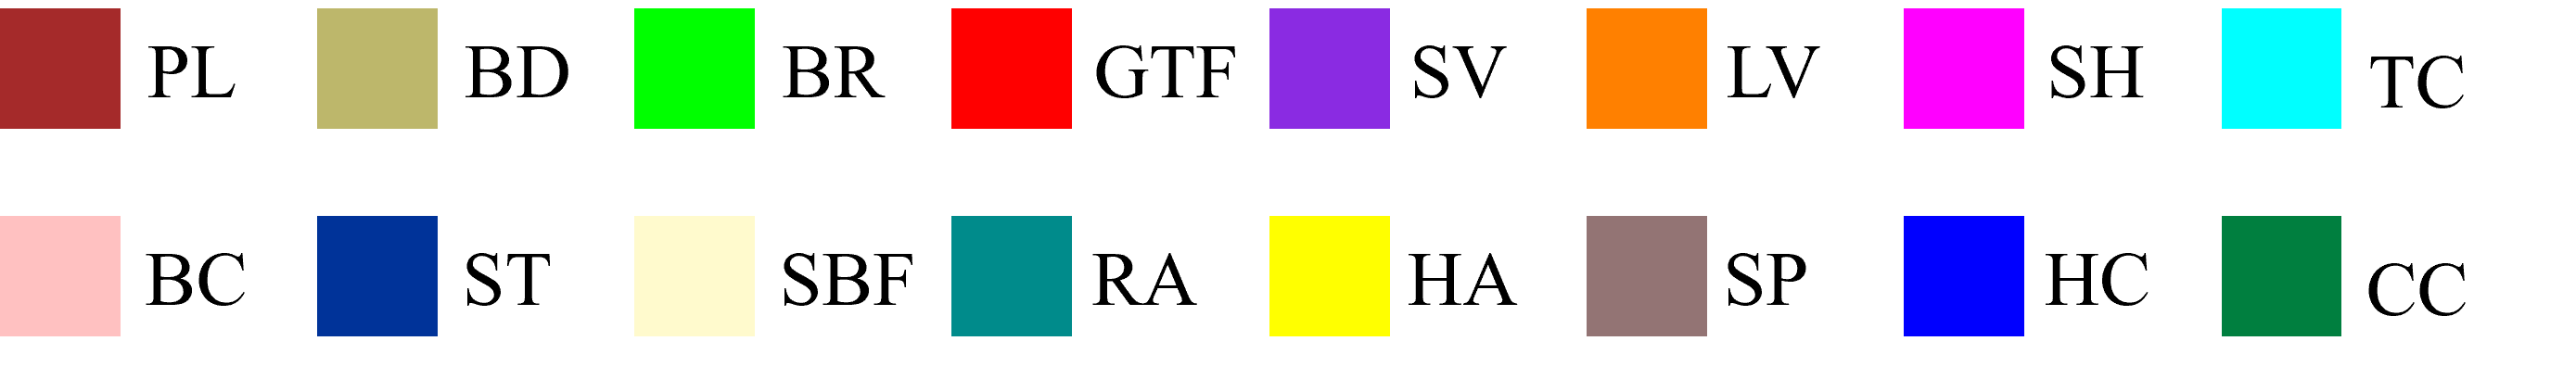}
        \caption*{}
        \label{fig:subdesc}
    \end{subfigure}
    \caption{Examples of detection results of ReDet and ReDet+\model. The color of the bounding boxes indicates the class of the objects, as specified in the legend.}
    \label{fig:main2}
\end{figure*}
